# Supplementary material for: CT to PET Translation: A Large-scale Dataset and Domain-Knowledge-Guided Diffusion Approach
Source: arXiv:2410.21932 source file (2024-10-29)
Supplement: Supplementary file 1 [file 6-Supplementary-Material.tex]

\section{Deduction Details of Brownian Bridge Diffusion Model}
\noindent \textbf{Forward Process.}
We utilize the sample forwarding process outlined in \cite{li2023bbdm}.
Starting from an initial state $\boldsymbol{x}_0$ and aiming for a destination state $\boldsymbol{y}$, the intermediate state $\boldsymbol{x}_t$ at timestep $t$ can be computed in discrete form as $\boldsymbol{x}_t=\left(1-m_t\right) \boldsymbol{x}_0+m_t \boldsymbol{y}+\sqrt{\delta_t} \epsilon_t$. Here, $m_t = t / T$, where $T$ represents the total number of steps in the diffusion process, $\delta_t$ indicates the variance of the original Brownian bridge, and $\epsilon$ depicts a Gaussian noise, i.e., $\epsilon \sim \mathcal{N}(\mathbf{0}, \mathbf{I})$. The forward process can be defined as: 
\begin{equation}
\label{eq:forward_diffusion}
    q_{BB} \left( \boldsymbol{x}_t | \boldsymbol{x}_0, y) = \mathcal{N} (\boldsymbol{x}_t; (1 - m_t) \boldsymbol{x}_0 + m_t \boldsymbol{y}, \delta_t \mathbf{I} \right).
\end{equation}
Throughout the training phase, we employ the following formula to establish the transition probability between two consecutive steps: \\
%Equation~\ref{eq:transition_probability} to establish the transition probability between two consecutive steps.
% , with $\boldsymbol{x}_{t-1} = \left(1-m_{t-1}\right) \boldsymbol{x}_0+m_t \boldsymbol{y}+\sqrt{\delta_{t-1}} \epsilon_{t-1}$.
\scalebox{0.9}{
\begin{minipage}{0.52\textwidth}
\begin{align}
\label{eq:transition_probability}
    q_{BB} (\boldsymbol{x}_t | \boldsymbol{x}_{t-1}, \boldsymbol{y}) &= \mathcal{N} \left( \boldsymbol{x}_t;  \frac{1 - m_t}{ 1 - m_{t-1} } \boldsymbol{x}_{t-1} \right. \nonumber \\ 
    &\left. + \left(m_t - \frac{1 - m_t}{ 1 - m_{t-1}} m_{t-1}\right) \boldsymbol{y}, \delta_{t|t-1} \mathbf{I} \right), \nonumber \\
    \text{with} \quad \delta_{t \mid t-1} &= \delta_t - \delta_{t-1} \frac{\left(1 - m_t\right)^2}{\left(1 - m_{t-1}\right)^2}.
\end{align}
\end{minipage}
}

% where $\delta_{t|t-1}$ is calculated by $\delta_t$ as 
\noindent \textbf{Reverse Process.} 
The reverse initiates by conditionally assigning $\boldsymbol{x}_T = \boldsymbol{y}$. Furthermore, to incorporate the domain knowledge, we integrate the Attention map $\boldsymbol{M}_\sigma$ and the Attenuation map $\boldsymbol{M}_\mu$ within the hidden state $\boldsymbol{x}_t$ at every timestep $t$ as follows: \\
\scalebox{0.86}{
\begin{minipage}{0.55\textwidth}
\begin{align}
    p_\theta(\boldsymbol{x}_{t-1} | \boldsymbol{x}_t, \boldsymbol{M}_\sigma, \boldsymbol{M}_\mu, \boldsymbol{y}) =&~ \mathcal{N} (\boldsymbol{x}_{t-1}; \mu_\theta (\boldsymbol{x}_t, \boldsymbol{M}_\sigma, \boldsymbol{M}_\mu, \boldsymbol{y}, t ), \tilde{\delta}_t \mathbf{I}), \nonumber \\
   \mu_\theta (\boldsymbol{x}_t, \boldsymbol{M}_\sigma, \boldsymbol{M}_\mu, \boldsymbol{y}, t) =&~ c_{x t} \boldsymbol{x}_t + c_{y t} \boldsymbol{y} \nonumber \\ 
   + & c_{\epsilon t} \boldsymbol{\epsilon}_\theta (\text{concat}(\boldsymbol{x}_t, \boldsymbol{M}_\sigma, \boldsymbol{M}_\mu), t), 
\label{eq:reverse_process}
\end{align}
\end{minipage}
}

where $\mu_\theta (\boldsymbol{x}_t, \boldsymbol{M}_\sigma, \boldsymbol{M}_\mu, \boldsymbol{y}, 
t)$ represents the predicted mean and $\tilde{\delta}_t$ represents the variance of the distribution at time step $t$.

\noindent \textbf{Training Objective.} 
The training of CPDM involves optimizing the following ELBO:

\scalebox{0.86}{
\begin{minipage}{0.55\textwidth}
\centering
\begin{equation*}
    \begin{aligned}
        &\text{ELBO} = -\mathbb{E}_q\left(D_{K L}\left(q_{B B}\left(\boldsymbol{x}_T \mid \boldsymbol{x}_0, \boldsymbol{y}\right) \|  
        p\left(\boldsymbol{x}_T \mid \boldsymbol{M}_\sigma, \boldsymbol{M}_\mu, \boldsymbol{y}\right)\right)\right. \\
        & +\sum_{t=2}^T D_{K L}\left(q_{B B}\left(\boldsymbol{x}_{t-1} \mid \boldsymbol{x}_t, \boldsymbol{x}_0, \boldsymbol{y}\right) \| p_\theta\left(\boldsymbol{x}_{t-1} \mid \boldsymbol{x}_t, \boldsymbol{M}_\sigma, \boldsymbol{M}_\mu, \boldsymbol{y}\right)\right)  
         \\
        & \left.-\log p_\theta\left(\boldsymbol{x}_0 \mid \boldsymbol{x}_1, \boldsymbol{M}_\sigma, \boldsymbol{M}_\mu, \boldsymbol{y}\right)\right).
    \end{aligned}
\end{equation*}
\end{minipage}
}

By integrating Equation~\ref{eq:forward_diffusion} and Equation~\ref{eq:transition_probability}, $q_{B B}\left(\boldsymbol{x}_{t-1} \mid \boldsymbol{x}_t, \boldsymbol{x}_0, \boldsymbol{y}\right)$ of the second term can be derived using Bayes' theorem and the Markov chain property: \\
\scalebox{0.86}{
\begin{minipage}{0.55\textwidth}
\begin{equation}
    \begin{aligned}
        q_{B B}\left(\boldsymbol{x}_{t-1} \mid \boldsymbol{x}_t, \boldsymbol{x}_0, \boldsymbol{y}\right) & =\frac{q_{B B}\left(\boldsymbol{x}_t \mid \boldsymbol{x}_{t-1}, \boldsymbol{y}\right) q_{B B}\left(\boldsymbol{x}_{t-1} \mid \boldsymbol{x}_0, \boldsymbol{y}\right)}{q_{B B}\left(\boldsymbol{x}_t \mid \boldsymbol{x}_0, \boldsymbol{y}\right)} \\ 
        &=\mathcal{N}\left(\boldsymbol{x}_{t-1} ; \tilde{\boldsymbol{\mu}}_t\left(\boldsymbol{x}_t, \boldsymbol{x}_0, \boldsymbol{y}\right), \tilde{\delta}_t \boldsymbol{I}\right),
    \end{aligned}
\end{equation}
\end{minipage}
}

where the mean and variance term can be represented as:
\scalebox{0.86}{
\begin{minipage}{0.55\textwidth}
\begin{equation}
\label{eq:mean_forward}
\begin{aligned} \tilde{\boldsymbol{\mu}}_t\left(\boldsymbol{x}_t, \boldsymbol{x}_0, \boldsymbol{y}\right) &= \frac{\delta_{t-1}}{\delta_t} \frac{1-m_t}{1-m_{t-1}} \boldsymbol{x}_t +\left(1-m_{t-1} \frac{\delta_{t \mid t-1}}{\delta_t}\right) \boldsymbol{x}_0 \\
&+ \left(m_{t-1}-m_t \frac{1-m_t}{1-m_{t-1}} \frac{\delta_{t-1}}{\delta_t}\right) \boldsymbol{y}, \\
\end{aligned}
\end{equation}

\begin{equation}
\tilde{\delta}_t=\frac{\delta_{t \mid t-1} \cdot \delta_{t-1}}{\delta_t}.
\end{equation}
\end{minipage}
}

As $\boldsymbol{x_0}$ remains unknown during the inference stage, $\tilde{\boldsymbol{\mu}}_t$ can be reformulated by employing a reparametrization method combining Equation~\ref{eq:forward_diffusion} and Equation~\ref{eq:mean_forward}: 
\scalebox{0.86}{
\begin{minipage}{0.55\textwidth}
\begin{equation}
\tilde{\boldsymbol{\mu}}_t\left(\boldsymbol{x}_t, \boldsymbol{y}\right)=c_{x t} \boldsymbol{x}_t+c_{y t} \boldsymbol{y}+c_{\epsilon t}\left(m_t\left(\boldsymbol{y}-\boldsymbol{x}_0\right)+\sqrt{\delta_t} \boldsymbol{\epsilon}\right),
\end{equation}
\end{minipage}
}
whereas:
\scalebox{0.86}{
\begin{minipage}{0.45\textwidth}
\begin{equation}
    \begin{aligned}
        & c_{x t}=\frac{\delta_{t-1}}{\delta_t} \frac{1-m_t}{1-m_{t-1}}+\frac{\delta_{t \mid t-1}}{\delta_t}\left(1-m_{t-1}\right), \\
        & c_{y t}=m_{t-1}-m_t \frac{1-m_t}{1-m_{t-1}} \frac{\delta_{t-1}}{\delta_t}, \\
        & c_{\epsilon t}=\left(1-m_{t-1}\right) \frac{\delta_{t \mid t-1}}{\delta_t}.
    \end{aligned}
\end{equation}
\end{minipage}
}

Therefore, instead of predicting $\boldsymbol{x_0}$, we simply train a neural network $\epsilon_\theta$ to predict the noise. Consequently, $\boldsymbol{\mu}_{\boldsymbol{\theta}}$ can be represented as a linear combination of $\boldsymbol{x}_t, \boldsymbol{y}$, and the predicted noise $\boldsymbol{\epsilon}_\theta$ as follows: \\
\scalebox{0.86}{
\begin{minipage}{0.55\textwidth}
\begin{align}
\boldsymbol{\mu}_{\boldsymbol{\theta}}\left(\boldsymbol{x}_t, \boldsymbol{M}_\sigma, \boldsymbol{M}_\mu, \boldsymbol{y}, t\right)=&~c_{x t} \boldsymbol{x}_t+c_{y t} \boldsymbol{y} \nonumber \\
+ & c_{\epsilon t} \boldsymbol{\epsilon}_\theta\left(\text{concat}(\boldsymbol{x}_t, \boldsymbol{M}_\sigma, \boldsymbol{M}_\mu), t\right),
\end{align}
\end{minipage}
}

where $\text{concat}(\cdot)$ is the function of channel-wise concatenation.

Finally, the objective function obtained after simplifying the ELBO is decribed as Equation~\ref{eq:ELBO}: \\
\scalebox{0.82}{
\begin{minipage}{0.5\textwidth}
\begin{equation}
\label{eq:ELBO}
    \mathbb{E}_{\boldsymbol{x}_0, \boldsymbol{y}, \boldsymbol{\epsilon}}\left[c_{\epsilon t}\left\|m_t\left(\boldsymbol{y}-\boldsymbol{x}_0\right)+\sqrt{\delta_t} \epsilon - \epsilon_\theta\left(\text{concat}(\boldsymbol{x}_t, \boldsymbol{M}_\sigma, \boldsymbol{M}_\mu), t\right)\right\|^2\right].
\end{equation}
\end{minipage}
}

Algorithm~\ref{alg:training_proposed_model} shows the detailed implementation of the training process. 

\begin{algorithm}[t] \caption{CPDM Training Process}\label{alg:training_proposed_model} \begin{algorithmic}[1] \small \REPEAT \STATE Paired data: PET image $\boldsymbol{x_0} \sim q(\boldsymbol{x_0})$, CT image $\boldsymbol{y} \sim q(\boldsymbol{y})$; Attention map $\boldsymbol{M_\sigma}$; Attenuation map $\boldsymbol{M_\mu}$ \STATE Timestep \scalebox{0.9}{$t \sim Uniform(1, \dots, T)$} \STATE Gaussian noise \scalebox{0.9}{$\epsilon \sim \mathcal{N}(\mathbf{0}, \mathbf{I})$} \STATE Forward diffusion \scalebox{0.9}{$\boldsymbol{x_t} =\left(1-m_t\right) \boldsymbol{x_0} +  m_t  \boldsymbol{y}+\sqrt{\delta_t} \epsilon$} \STATE Take gradient descent: \\ \scalebox{0.9}{$\nabla_\theta\left\|m_t\left(\boldsymbol{y} - \boldsymbol{x_0} \right)+\sqrt{\delta_t} \epsilon - \epsilon_\theta \left(\text{concat}(\boldsymbol{x_t}, \boldsymbol{M_\sigma}, \boldsymbol{M_\mu}), t\right)\right\|_1$} \normalsize \UNTIL{converged} \normalsize \end{algorithmic} \end{algorithm}

For the sampling, we adopt the basic idea of DDIM (Denoising Diffusion Implicit Models)~\cite{song2020denoising}, where acceleration is achieved through a non-Markovian process. 
This approach ensures the preservation of the same marginal distributions found in Markovian inference processes, as outlined in Algorithm~\ref{alg:sampling_proposed_model}.

\begin{algorithm}[t]
\caption{CPDM Sampling Process}\label{alg:sampling_proposed_model}
\begin{algorithmic}[1]
\small
\STATE Sample conditional input: CT image $\boldsymbol{x_T} = \boldsymbol{y} \sim q(\boldsymbol{y})$; \\ Attention map $\boldsymbol{M_\sigma}$; Attenuation map $\boldsymbol{M_\mu}$ 
\FOR{$t=T, \ldots, 1$}
    \STATE \scalebox{0.86}{$\boldsymbol{z} \sim \mathcal{N}(\mathbf{0}, \mathbf{I})$ if $t>1$, else $\boldsymbol{z} = \mathbf{0}$}
    \STATE \scalebox{0.86}{$\boldsymbol{x_{t-1}} =  c_{xt} \boldsymbol{x_t} + c_{yt}\boldsymbol{y} -c_{\epsilon t} \epsilon_\theta\left(\text{concat}(\boldsymbol{x_t}, \boldsymbol{M_\sigma}, \boldsymbol{M_\mu}), t\right)+\sqrt{\tilde{\delta}_t} \boldsymbol{z} $}
\ENDFOR
\RETURN $\boldsymbol{x_0}$
\normalsize
\end{algorithmic}
\end{algorithm}

\section{Experiments Details}
\subsection{System Detail}
Experiments are performed on a machine equipped with an EPYC7402P AMD CPU and an NVIDIA A6000 GPU.

\subsection{Hyper-parameters}
In this section, we provide further implementation details for CPDM and other methods.

\subsubsection{CPDM (\textbf{Our proposed model})} 
We implement the CPDM as detailed in Section 4, utilizing the VQGAN~\cite{esser2021taming} for encoding and decoding CT and PET images, respectively.
In CPDM, the diffusion timesteps of the Brownian Bridge are set at $1000$ for training and reduced to $200$ for inference, aiming to balance quality and speed.

\textbf{VQGAN.} We retrain the VQGAN model used in BBDM~\cite{li2023bbdm} and LDM~\cite{rombach2022high} on the CT2PET dataset, using the same training set as the diffusion model in CPDM. With a downsampling factor of $f = 4$, both CT and PET images, originally of size $256 \times 256 \times 1$, are encoded into a latent space with dimensions $64 \times 64 \times 3$. 

\textbf{Segmentation Model.} a U-Net architecture~\cite{ronneberger2015u} with a pre-trained ResNet50 as its backbone for extracting the Attention map. The model takes a CT image input of resolution $256 \times 256 \times 1$ and outputs a soft mask that highlights the region of interest. The network is trained using the Dice Loss~\cite{milletari2016v} function, with the following hyperparameters: 100 total training epochs, the Adam optimizer with a learning rate of 0.0001, and no weight decay. Model checkpoints are saved based on the Intersection over Union (IoU) performance on the validation set.
 
\textbf{Denoising Network.} For a fair comparison in the latent space diffusion process, we adopt the same denoising network architecture as BBDM~\cite{li2023bbdm} and LDM~\cite{rombach2022high}. The architectural details are provided in Table~\ref{tab:config}.

\begin{table}[t]
\centering
\caption{Hyperparameters for CPDM.}
\label{tab:config}
\begin{tabular}{l|l}
\toprule
\textbf{Hyperparameters} & \textbf{Values} \\ 
\midrule
\textbf{Denoising Network} &  \\ 
% Input shape & $64 \times 64 \times 3$ \\ 
Channel multiplier & 1, 2, 3, 4 \\ 
\# Residual blocks per downsample & 2 \\
Attention resolutions & 32, 16, 8 \\ 
Channels & 128 \\ 
\# Parameters & 97.39M \\ 
\midrule
\textbf{EMA} &  \\ 
Start step & 30,000 \\ 
Decay & 0.995 \\ 
Update interval & 16 \\ 
Batch size & 16 \\ 
\midrule
\textbf{ReduceLROnPlateau Scheduler} &  \\ 
Max learning rate & $1.0 \times 10^{-4}$ \\ 
Min learning rate & $5.0 \times 10^{-7}$ \\ 
Factor & 0.5 \\ 
Patience & 3,000 \\ 
Cool down & 2,000 \\ 
Threshold & $1.0 \times 10^{-4}$ \\ 
\bottomrule
\end{tabular}
\end{table}

\textbf{Training Details.} To enhance model performance, we utilize Exponential Moving Average (EMA) alongside the ReduceLROnPlateau learning rate scheduler. The specific hyperparameter configurations are outlined in Table~\ref{tab:config}.

\textbf{Inference.} We perform inference with 200 steps, following the approach outlined in BBDM~\cite{li2023bbdm} and DDIM~\cite{song2020denoising}, as summarized in Algorithm~\ref{alg:sampling_proposed_model}.

% Denoising Network: 
%     input shape: $64 \times 64 \times 3$
%     channel multiplier: 1,2,3,4
%     attention resolutions: 32,16,8
%     channels: 128
%     # parameters: 234M
% EMA: 
%     start step: 30000
%     decay: 0.995
%     update interval: 16
%     batch size: 16
% ReduceLROnPlateau scheduler: 
%      max learning rate: $1.0e-4$
%      min learning rate: $5.0e-7$
%      factor: 0.5
%      patience: 3000
%      cool down: 2000
%      threshold: $1.0e-4$

\subsubsection{Pix2Pix}
Pix2Pix~\cite{isola2017image} is a supervised GAN model for paired image-to-image translation. The generator is a ResNet with 9 residual blocks, while the discriminator uses a 70x70 PatchGAN~\cite{isola2017image}. Training is conducted for 100 epochs with a learning rate of $2 \times 10^{-4}$, decaying linearly over another 100 epochs. The least-squares GAN loss (LSGAN) is applied, with instance normalization used in both the generator and discriminator. Adam optimizer with $\beta_1 = 0.5$ is employed, and a buffer of 50 images is used to stabilize training. The implementation is based on the code available at \url{https://github.com/junyanz/pytorch-CycleGAN-and-pix2pix}

\subsubsection{MedGAN}
MedGAN~\cite{armanious2020medgan} is a GAN model that integrates the adversarial framework with a novel combination of non-adversarial losses. The model is optimized using the Adam optimizer with a momentum value of 0.5 and a learning rate of 0.0001. Instance normalization is applied with a batch size of 1. The generator adopts a U-Net~\cite{ronneberger2015u} architecture, while the patch-based discriminator is updated once for every three generator training iterations. The implementation is based on a modified version of the UP-GAN framework, where we utilize one GAN block and replace the 3-head U-Net architecture with a single-head U-Net.  

\subsubsection{UP-GAN} 
UP-GAN~\cite{upadhyay2021uncertainty} is a GAN model that leverages an uncertainty-guided progressive learning scheme for image-to-image translation. The architecture consists of two GAN blocks, both initialized using the progressive learning strategy, with loss weights \(\lambda_1 = 1\) and \(\lambda_2 = 0.001\). The model is optimized using the Adam optimizer, with hyperparameters \(\beta_1 = 0.9\), \(\beta_2 = 0.999\). During initialization, the learning rate is set to 0.0001, followed by an increase to 0.0005 post-initialization, and decays via cosine annealing over 200 epochs per GAN block (a total of 400 epochs). Training is conducted with a batch size of 1. The implementation is based on the code available at 
\url{https://github.com/ExplainableML/UncerGuidedI2I.git}

\subsubsection{DDIB} 
DDIB~\cite{su2022dual} is an image translation method built upon recent advances in score-based diffusion models, theoretically grounded as Schrödinger Bridges in the image space. Both the source (CT) and target (PET) synthetic models are trained with identical settings: 1000 diffusion steps, using the Adam optimizer with a learning rate of 0.0001 and no weight decay, a batch size of 32, and a total of 250,000 iterations. The implementation is based on the code available at \url{https://github.com/suxuann/ddib}
\subsubsection{Palette} 
Palette~\cite{saharia2022palette} is an image-to-image diffusion model that employs exponential moving average (EMA) from the first iteration with a decay rate of 0.9999 for stable training. The Adam optimizer is used with a learning rate of $5 \times 10^{-5}$ and no weight decay. The beta schedule during training follows a linear progression over 2000 timesteps, starting at $1 \times 10^{-6}$ and gradually increasing to 0.01. Inference is performed over 1000 steps. The implementation is based on the code available at \url{https://github.com/Janspiry/Palette-Image-to-Image-Diffusion-Models}

\subsubsection{LDM}
LDM~\cite{rombach2022high} utilizes conditional diffusion models for image translation in the VQGAN latent space. For a fair comparison, we use the same retrained VQGAN and denoising architecture as in CPDM. The model is optimized using Adam, with a learning rate of $1 \times 10^{-4}$ and $\beta_1 = 0.9$. A learning rate scheduler is applied, with a cooldown of 3000 steps, a decay factor of 0.5, and a minimum learning rate of $5 \times 10^{-7}$. An exponential moving average (EMA) with a decay of 0.995 is introduced after 30,000 steps. Training involves 1000 diffusion steps, while the inference process uses 200 steps, leveraging the DDIM~\cite{song2020denoising} algorithm. The implementation is based on the code available at \url{https://github.com/CompVis/latent-diffusion.git}
\subsubsection{SDEdit}
SDEdit~\cite{meng2021sdedit} is a diffusion-based image-to-image translation method that operates in the latent space of VQGAN, built on Hugging Face's Stable Diffusion framework. For a fair comparison, we use the same retrained VQGAN and denoising architecture as in CPDM. The diffusion model is trained using the DDPM approach. During inference, the reverse stochastic differential equation (SDE) is solved starting from an intermediate time step, $t_0 = 400/1000 = 0.4$, out of a total of 1000 steps. The implementation is based on the code available at \url{https://github.com/ermongroup/SDEdit}

\subsubsection{BBDM}
BBDM~\cite{li2023bbdm} is a diffusion-based image-to-image translation model that frames the process as a stochastic Brownian bridge in the VQGAN latent space. For consistency, we use the same retrained VQGAN and denoising architecture as in CPDM. The model is optimized using the Adam optimizer with a learning rate of $1 \times 10^{-4}$ and $\beta_1 = 0.9$. The learning rate scheduler includes a cooldown period of 3000 steps, a decay factor of 0.5, and a minimum learning rate of $5 \times 10^{-7}$. An exponential moving average (EMA) with a decay rate of 0.995 is applied, starting after 30,000 steps. Training involves 1000 diffusion steps, while inference is performed in 200 steps, using the DDIM~\cite{song2020denoising} algorithm. The implementation is based on the code available at \url{https://github.com/xuekt98/BBDM.git}

\subsection{Detail of the Evaluation Metrics}
Following~\cite{armanious2020medgan, upadhyay2021uncertainty}, we utilize Learned Perceptual Image Patch Similarity (LPIPS), Mean Absolute Error (MAE), Structural Similarity Index Measure (SSIM), and Peak Signal-to-Noise Ratio (PSNR) metrics to assess the quality of generated PET images. 
LPIPS evaluates perceptual similarity, which is crucial for capturing medical details. 
MAE measures the average error, indicating accuracy. 
SSIM reflects visual quality by assessing changes in the image structure, whereas PSNR gauges image fidelity. 

\subsubsection{Mean Absolute Error (MAE)} 
This metric measures the average absolute difference between the predicted values and the actual values for all data samples. MAE is commonly used to evaluate the performance of prediction models, especially in the fields of machine learning and computer vision. A lower MAE indicates that the model is more accurate on the test data. The formula for MAE is given by:

\[
\text{MAE} = \frac{1}{n} \sum_{i=1}^{n} | y_i - \hat{y}_i |
\]
where \( y_i \) is the actual value, \( \hat{y}_i \) is the predicted value, and \( n \) is the number of samples.

\subsubsection{Learned Perceptual Image Patch Similarity (LPIPS)}
This metric evaluates the perceptual similarity between two images by leveraging deep learning features. LPIPS is widely used in the assessment of image quality and the effectiveness of image generation models. It measures the distance between feature representations extracted from pre-trained neural networks, indicating how perceptually similar two images are to human observers. A lower LPIPS score suggests higher perceptual similarity. The formula for LPIPS is given by:
\[
\text{LPIPS} = \sum_{l} \frac{1}{H_l W_l} \sum_{h=1}^{H_l} \sum_{w=1}^{W_l} \| \phi_l(I_1)_{h,w} - \phi_l(I_2)_{h,w} \|_2
\]
where \( \phi_l \) denotes the feature map extracted by the neural network at layer \( l \), \( I_1 \) and \( I_2 \) are the two images being compared, \( H_l \) and \( W_l \) are the height and width of the feature map at layer \( l \), and \( \| \cdot \|_2 \) represents the Euclidean distance.

\subsubsection{Structural Similarity Index Measurement (SSIM)}
This is a visual metric used to assess the similarity between two images. SSIM is calculated based on three comparison parameters: (i) luminance, (ii) contrast, and (iii) structure. SSIM ranges from -1 to 1, with a value of 1 indicating that the two data sets are identical. Higher SSIM values correspond to better model performance. The formula for SSIM is given by:
\[
\text{SSIM}(x, y) = \frac{(2\mu_x \mu_y + c_1)(2\sigma_{xy} + c_2)}{(\mu_x^2 + \mu_y^2 + c_1)(\sigma_x^2 + \sigma_y^2 + c_2)}
\]
where \(\mu_x\) and \(\mu_y\) are the mean values of \(x\) and \(y\), \(\sigma_x^2\) and \(\sigma_y^2\) are the variances of \(x\) and \(y\), \(\sigma_{xy}\) is the covariance of \(x\) and \(y\), and \(c_1\) and \(c_2\) are constants to stabilize the division.

\subsubsection{Peak Signal-to-Noise Ratio (PSNR)}
This metric measures the ratio between the maximum possible power of a signal and the power of the noise that affects the accuracy of the signal, typically expressed in decibels (dB). In the context of evaluating the quality of generated images, a higher PSNR indicates better image quality. When two images are identical, the PSNR approaches infinity. Generally, if the PSNR value is 40 dB or higher, the human eye can hardly distinguish between the original and generated images. PSNR is defined as:
\[
\text{PSNR} = 10 \cdot \log_{10}\left(\frac{\text{MAX}^2}{\text{MSE}}\right)
\]
where \(\text{MAX}\) is the maximum possible pixel value of the image and \(\text{MSE}\) is the mean squared error between the original and generated images.

\begin{figure*}[t]
    \centering
    \begin{minipage}[t]{0.32\linewidth} % Adjust the width as needed
        \centering
        \includegraphics[width=1.0\linewidth]{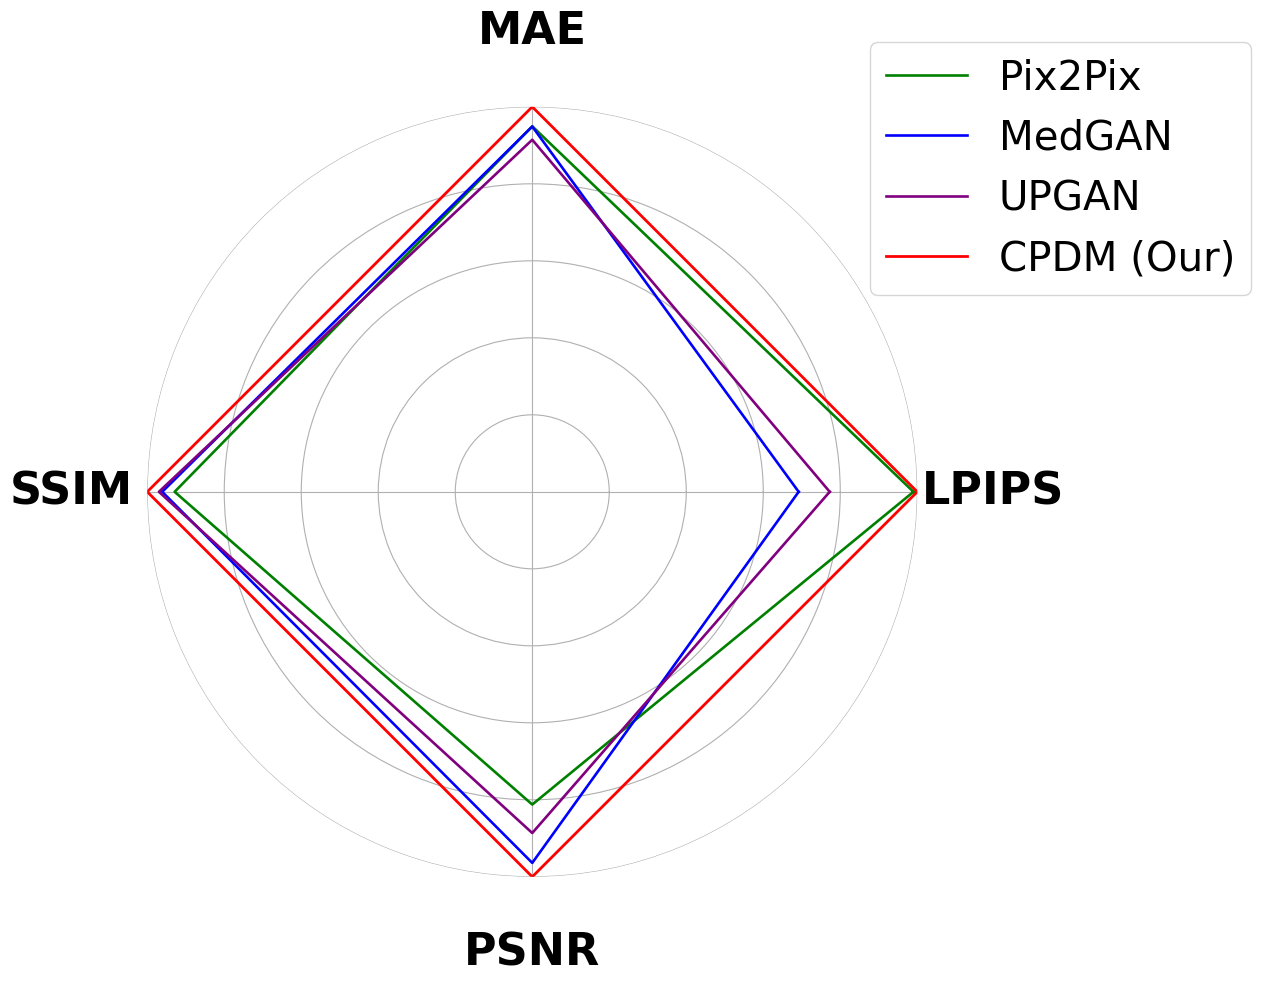}
        \caption{Comparison of CPDM (Our) with GAN-based Models.}  
        \label{fig:comparison_with_gans}
    \end{minipage}%
    \hfill % Adds space between the two minipages
    \begin{minipage}[t]{0.32\linewidth} % Adjust the width as needed
        \centering
        \includegraphics[width=1.1\linewidth]{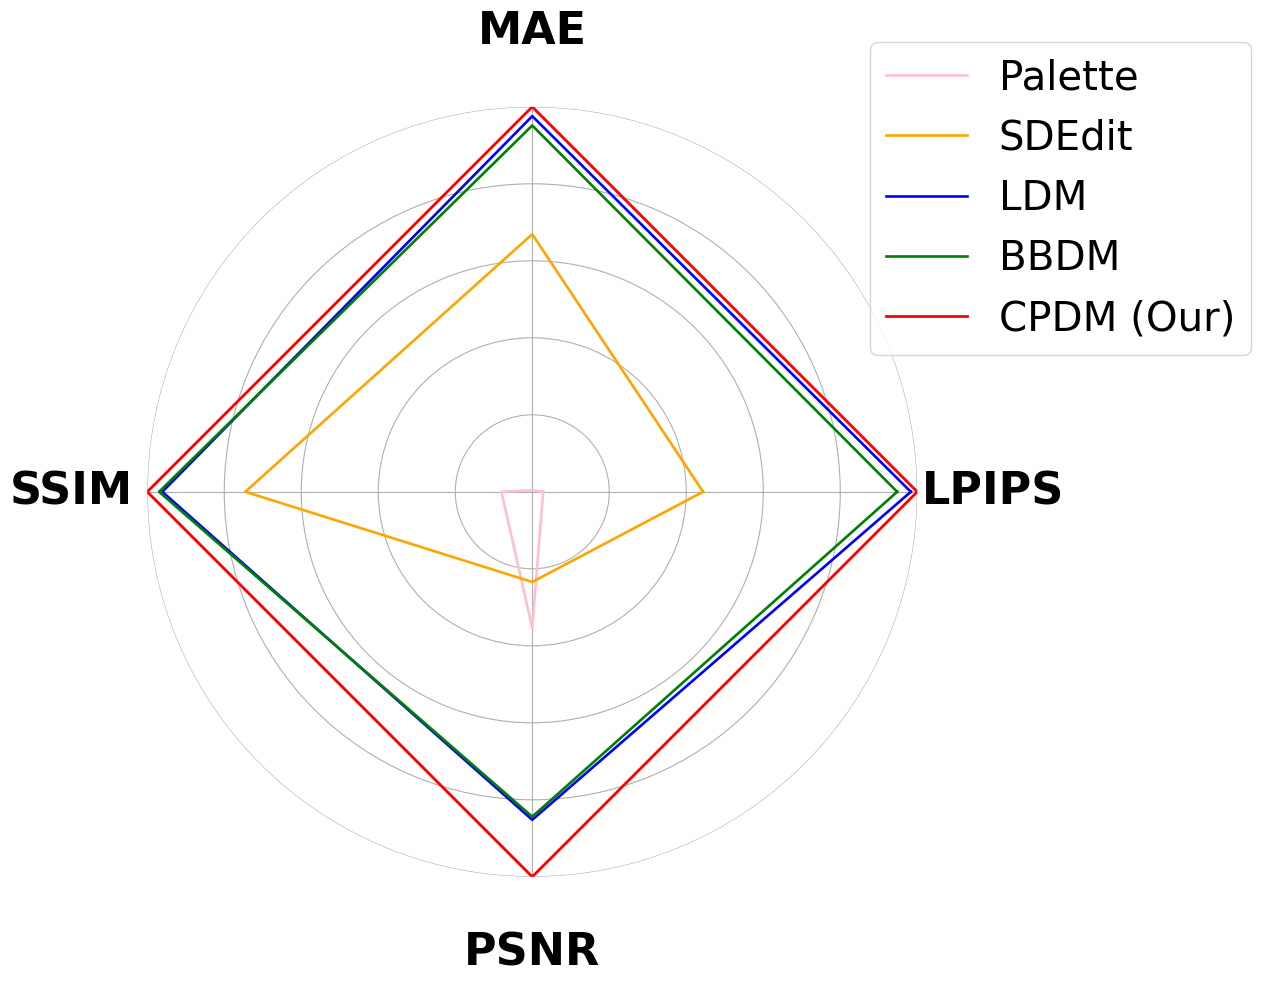}
        \caption{Comparison of CPDM (Our) with Diffusion-based Models.}  
        \label{fig:comparison_with_diffusion}
    \end{minipage}%
    \hfill % Adds space between the two minipages
    \begin{minipage}[t]{0.32\linewidth} % Adjust the width as needed
        \centering
        \includegraphics[width=1.0\linewidth]{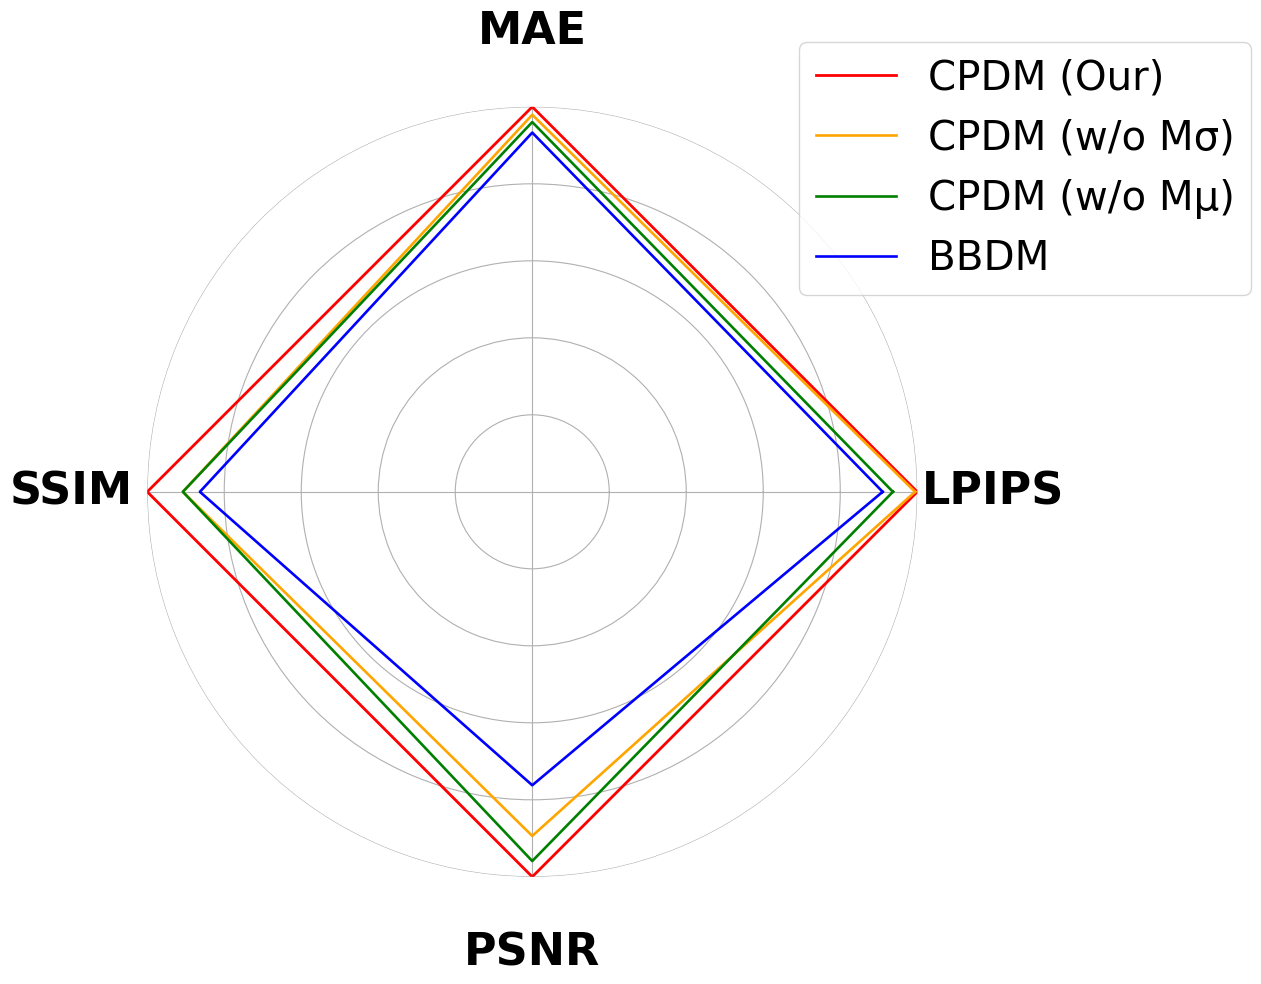}
        \caption{Comparison of CPDM (Our) with CPDM Variants.}  
        \label{fig:comparison_with_variants}
    \end{minipage}%
\end{figure*}

\section{Ablation Studies}
% \subsubsection{Convergence analysis}
% \truong{Move Figure 3 here! Add at least 1 GAN method and 1 diffusion method into Figure 3}
    % \begin{figure}[t]
    %     \centering
    %     \includegraphics[width=\linewidth]{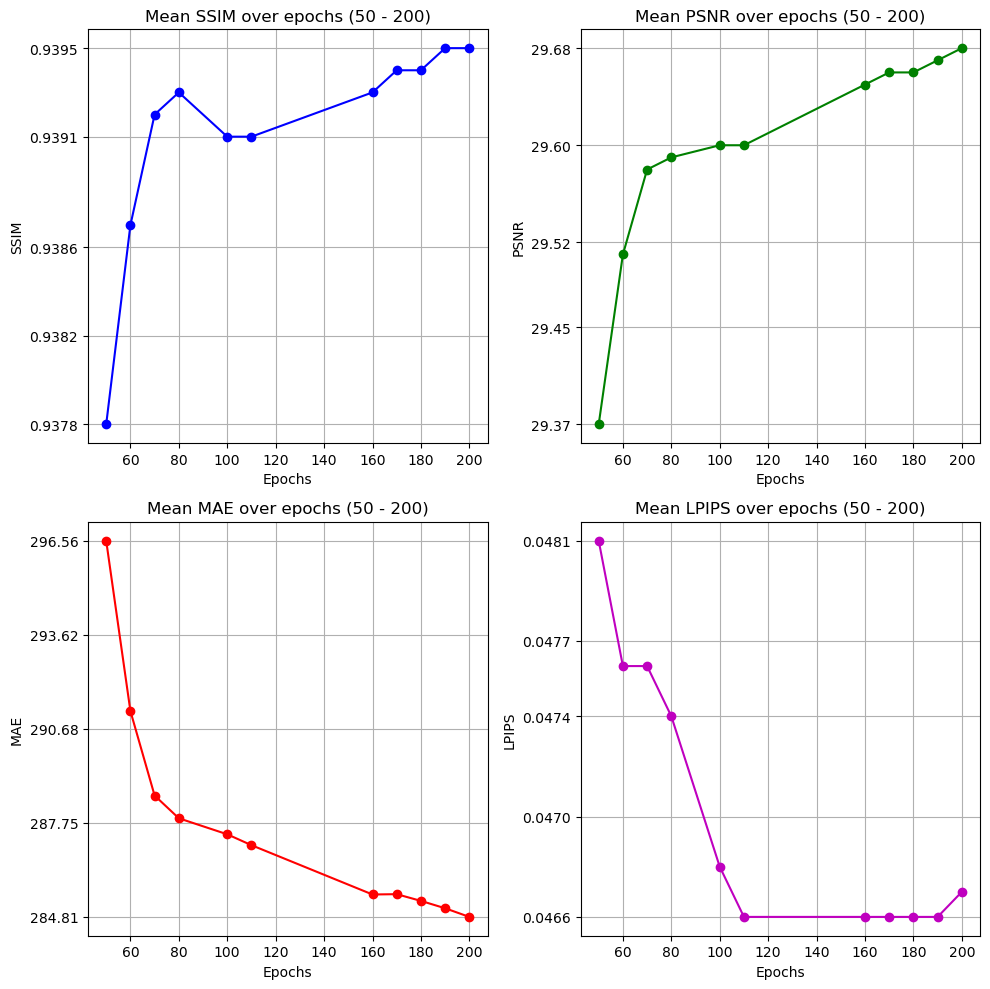}
    %     %\includegraphics[width=0.95\linewidth]{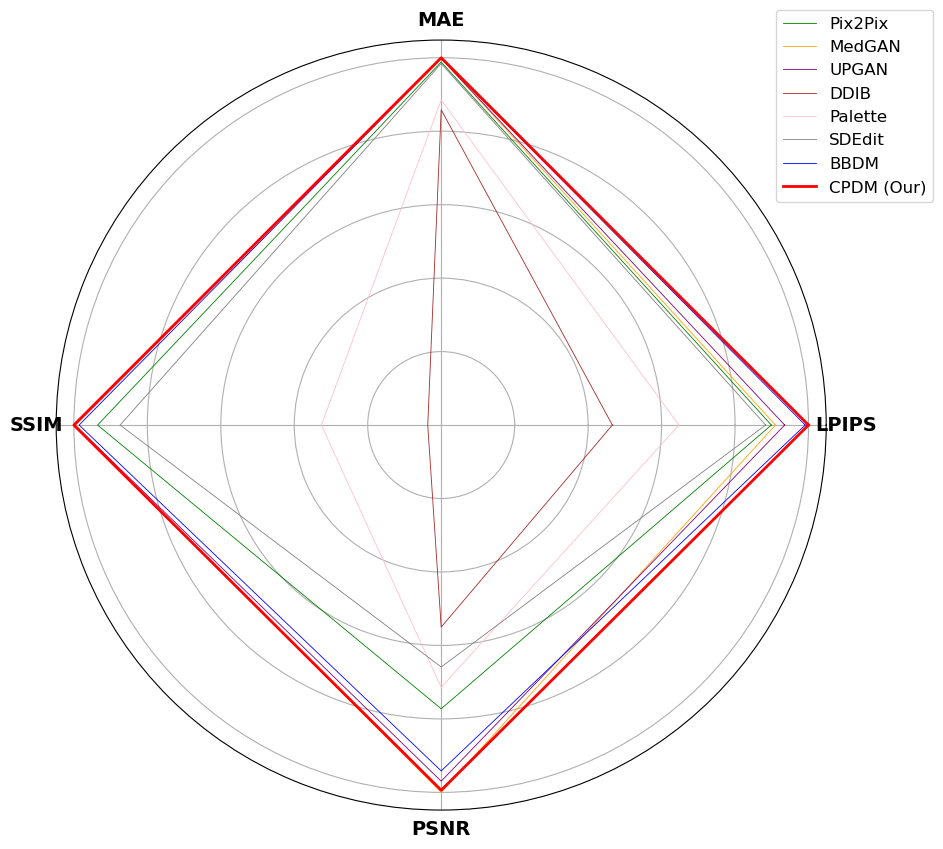}
    %     % The visualizations, moving from left to right, illustrate the early, middle, and final steps in the diffusion process from CT to PET.
    %     \caption{\truong{redraw the figures and organize it into 1 row format.} \label{fig:metrics}} 
    % \end{figure}
    % \hfill

\subsection{Analysis of the CPDM's Performance}
% \truong{Draw 3 radar figures. (1) Compare CPDM with GAN-based, (2) Compare CPDM with diffusion based method, (3) Compare CPDM with 2 other version of CPDM and BBDM.}
% \begin{figure}[t]
%     \centering
%     %\begin{minipage}[t]{0.45\textwidth} % Adjust the width as needed
%         \centering
%         \includegraphics[width=1.0\linewidth]{Figures/visualization/radar_chart.png}
%         \caption{Draw 3 other figure and organize it into 1 row format.}  
%         \label{fig:radar_chart}
%     %\end{minipage}%
%     %\hfill % Adds space between the two minipages
% \end{figure}

The performance of the CPDM model is evaluated and compared with several GAN-based, diffusion-based, and CPDM variant models using radar charts that visualize four key metrics: \textbf{LPIPS}, \textbf{MAE}, \textbf{SSIM}, and \textbf{PSNR}. Each group of models is analyzed separately to highlight the advantages and challenges of CPDM in different categories.

\textbf{Comparison with GAN-based Models.} The first radar chart compares CPDM with three GAN-based models: \textbf{Pix2Pix}, \textbf{MedGAN}, and \textbf{UP-GAN}. In Figure \ref{fig:comparison_with_gans}, CPDM shows superior performance across most metrics, particularly in LPIPS and SSIM, where the normalized values of CPDM are closer to the ideal value (1). While GAN-based models also perform well in terms of SSIM and MAE, CPDM demonstrates a more balanced performance across all metrics, showing its robustness.

\textbf{Comparison with Diffusion-based Models.} The second radar chart (Figure \ref{fig:comparison_with_diffusion}) illustrates the comparison between CPDM and several diffusion-based models: \textbf{Palette}, \textbf{SDEdit}, \textbf{LDM}, and \textbf{BBDM}. This figure highlights the strengths of CPDM in SSIM and PSNR, where it consistently outperforms the diffusion-based models. Moreover, models relying on conditional synthetic generation, such as Palette and SDEdit, show notably poor performance across most metrics, indicating the limitations of these approaches in handling the I2I translation task.

\textbf{Comparison with CPDM Variants.} In the third radar chart (Figure \ref{fig:comparison_with_variants}), CPDM is compared with its two variants CPDM (w/o $M_\sigma$) and CPDM (w/o $M_\mu$) as well as BBDM. The results show that the original CPDM performs better than its variants, where the impact of removing certain components from the model is clearly seen. The variants show a significant decrease in performance, especially in SSIM and PSNR, reaffirming the effectiveness of the original CPDM design in The variants show a significant decrease in performance, especially in SSIM, reaffirming the effectiveness of the original CPDM design in balancing both perceptual fidelity and image quality.

\subsection{Training Time}
Table \ref{tab:training_time} presents a comparison of the training times across different methods. The table reports the time per epoch, the total number of epochs, and the overall training time (in seconds). CPDM exhibits a competitive convergence time relative to other diffusion-based models, although it remains slower than GANs. This increased training time, however, reflects a trade-off that results in enhanced fidelity and image quality. Furthermore, diffusion models, including CPDM, tend to be easier to fine-tune and demonstrate more stable performance across diverse tasks, underscoring their robustness in generating high-quality images.
\begin{table}[tb]
\centering
\caption{Training time of different methods.} 
\label{tab:training_time}
% \setlength\tabcolsep{3pt} % default value: 6pt
%\resizebox{0.9\linewidth}{!}
{%
    \begin{tabular}{c|l||r|r|r}
        \toprule
        \multicolumn{2}{c||}{\textbf{Model}} & \textbf{\begin{tabular}[c]{@{}c@{}}Time per\\ epoch (s)\end{tabular}} 
        & \textbf{\begin{tabular}[c]{@{}c@{}}No. of\\ epochs\end{tabular}} 
        & \textbf{\begin{tabular}[c]{@{}c@{}}Total \\ time (s)\end{tabular}} \\
        \midrule
        \multirow{3}{*}{\rotatebox{90}{\textbf{GAN}}}  
        & Pix2Pix~\cite{isola2017image} & \multicolumn{1}{r|}{121} & \multicolumn{1}{r|}{100} & {12100} \\
        & MedGAN~\cite{armanious2020medgan} & \multicolumn{1}{r|}{864} & \multicolumn{1}{r|}{50} & 43200 \\
        & UP-GAN~\cite{upadhyay2021uncertainty} & \multicolumn{1}{r|}{861} & \multicolumn{1}{r|}{400} & 344400 \\ 
        \midrule
        \multirow{6}{*}{\rotatebox{90}{\textbf{Diffusion}}}  
        & DDIB~\cite{su2022dual} & \multicolumn{1}{r|}{16116} & \multicolumn{1}{r|}{75} & 1208700 \\
        & Palette~\cite{saharia2022palette} & \multicolumn{1}{r|}{911} & \multicolumn{1}{r|}{157} & 143027 \\
        & BBDM~\cite{li2023bbdm} & \multicolumn{1}{r|}{511} & \multicolumn{1}{r|}{112} & 57232 \\
        & SDEdit~\cite{meng2021sdedit} & \multicolumn{1}{r|}{520} & \multicolumn{1}{r|}{200} & 104000 \\
        & LDM~\cite{rombach2022high} & \multicolumn{1}{r|}{525} & \multicolumn{1}{r|}{200} & 105000 \\
        & \textbf{CPDM} (Our) & \multicolumn{1}{r|}{526} & \multicolumn{1}{r|}{200} & 105200 \\
        \bottomrule
    \end{tabular}
}              
\end{table}

\begin{figure*}[th]
    \centering
    \includegraphics[width=1.0\linewidth]{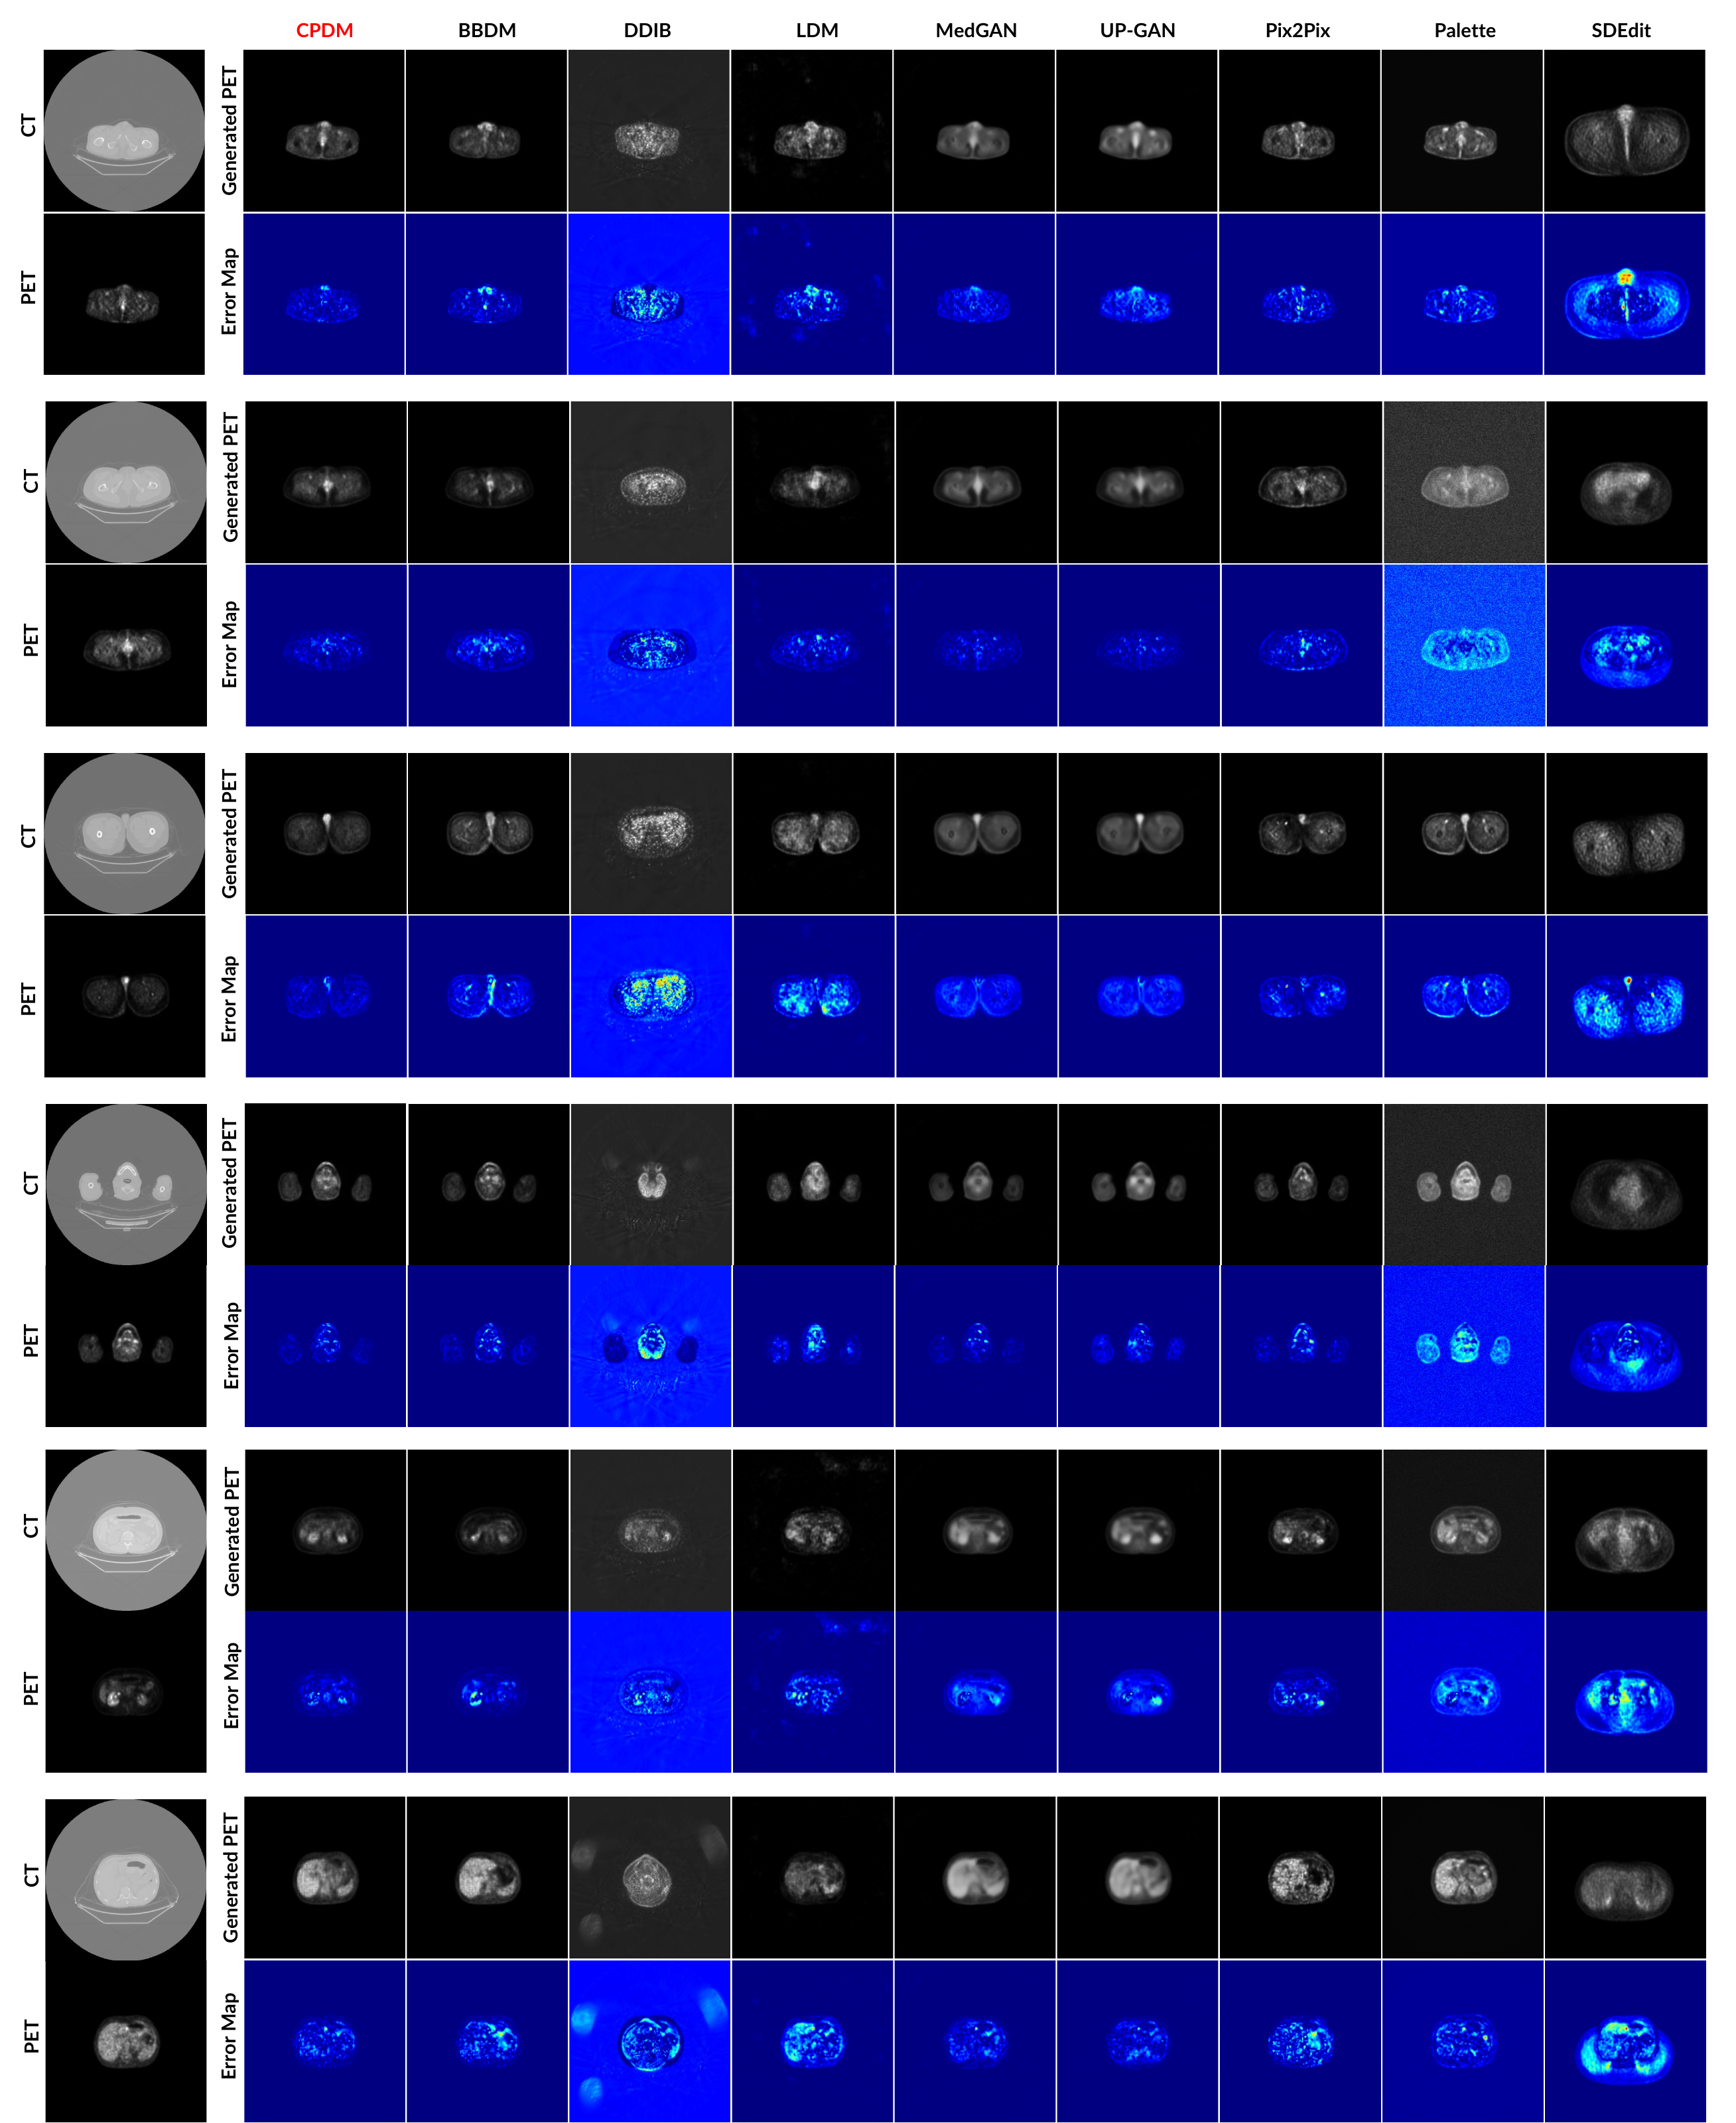}
        \caption{Visualization of PET images generated by different methods across various anatomical regions.}
   \label{fig:visualization_appendix_1}
\end{figure*}

\begin{figure*}[t]
    \centering
    \includegraphics[width=1.0\linewidth]{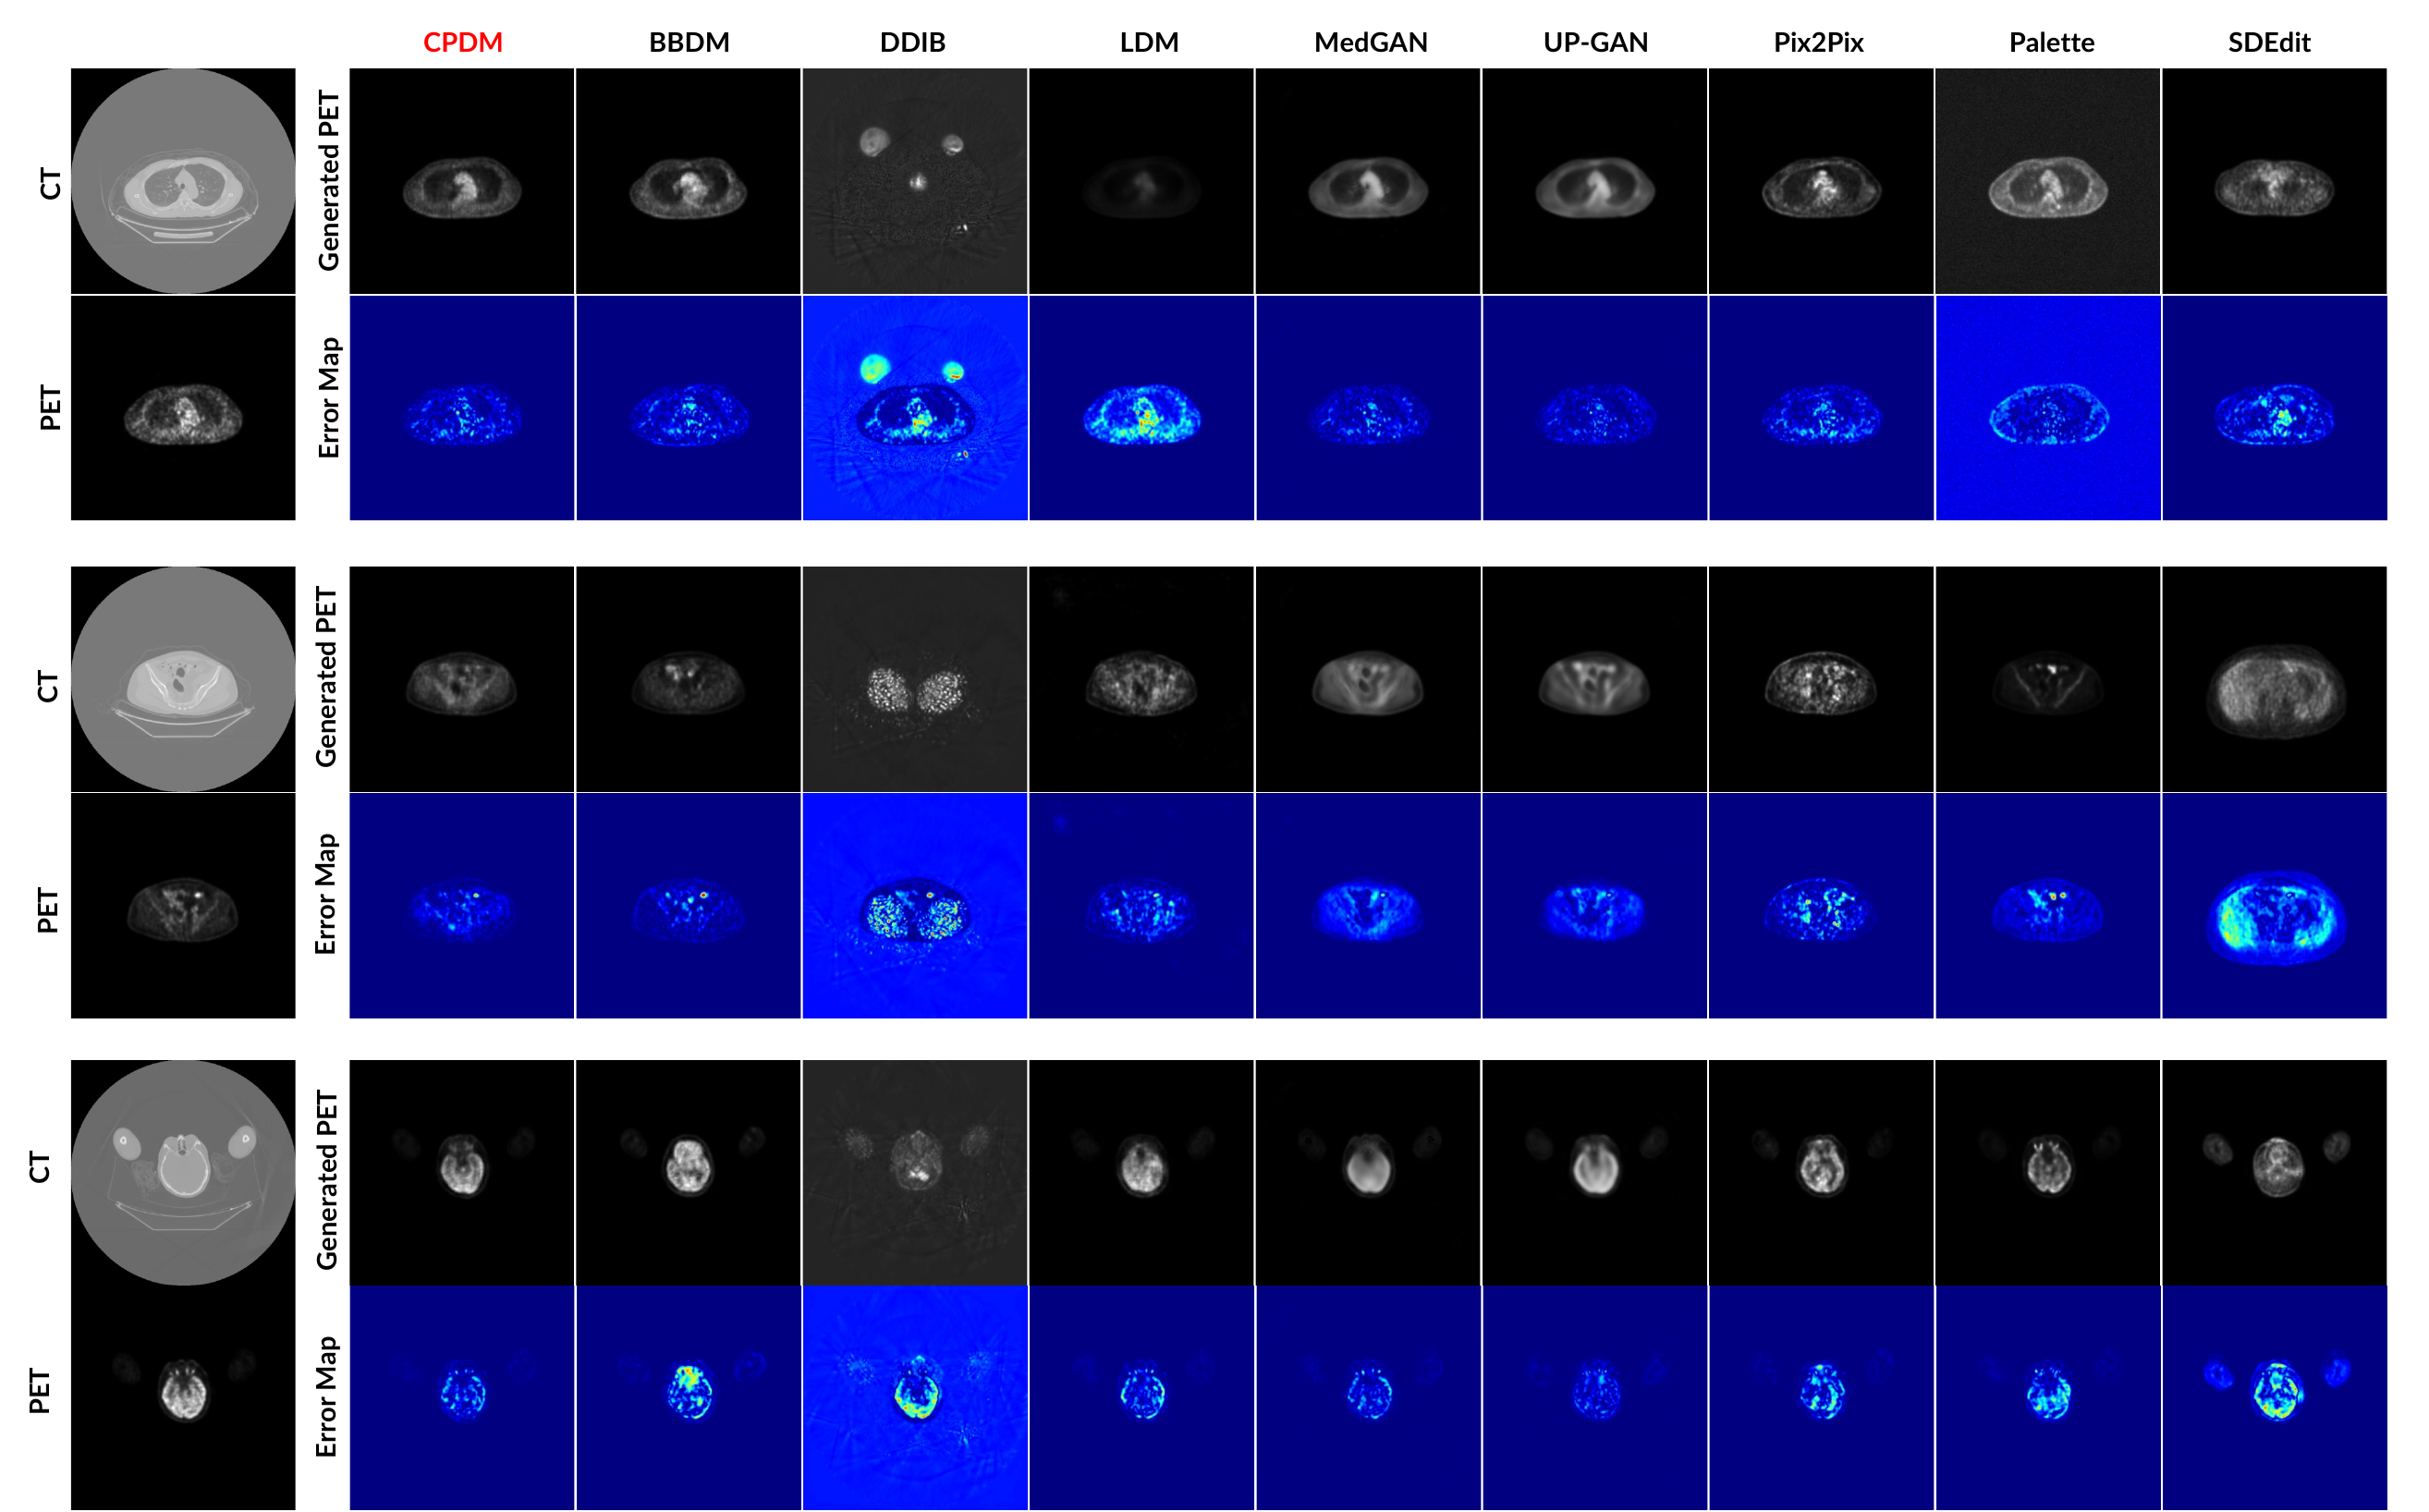}
        \caption{Visualization of PET images generated by different methods across various anatomical regions.}
   \label{fig:visualization_appendix_3}
\end{figure*}

\begin{figure*}[t]
    \centering
    \includegraphics[width=0.93\linewidth]{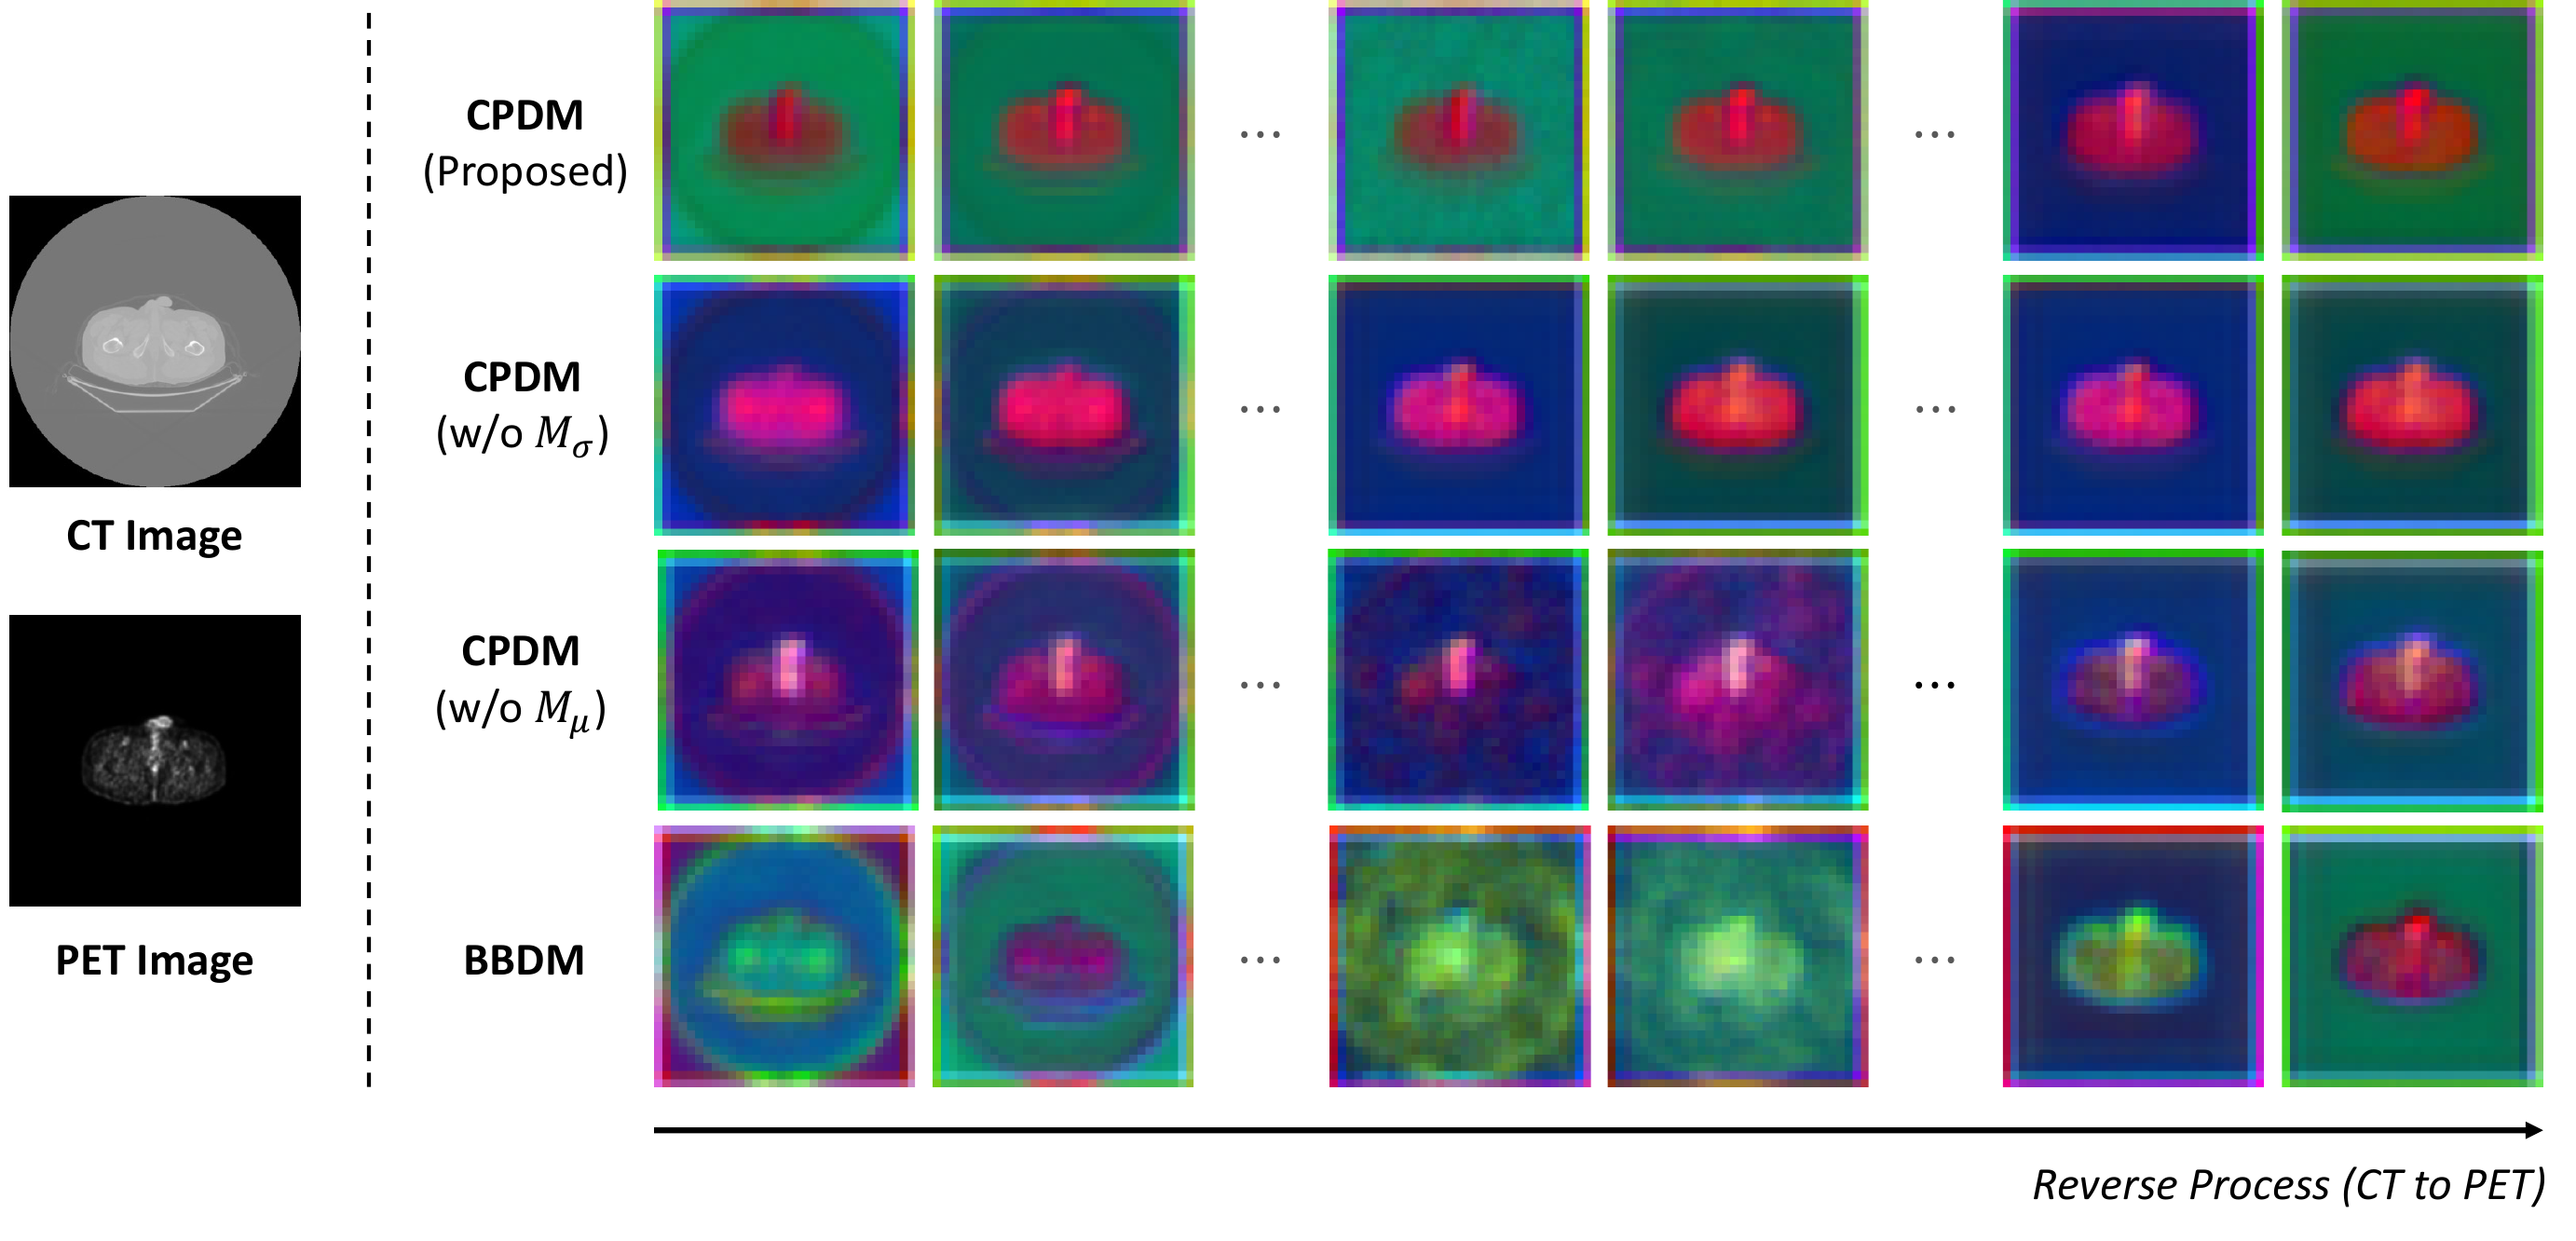}
     \caption{\textbf{PCA visualization of spatial features extracted from the denoising network.} The grayscale images on the left show the ground-truth paired CT-PET images. The visualizations, from left to right, illustrate the early, middle, and final steps in the diffusion process from CT to PET. Images produced by CPDM focus on the region of interest, whereas those generated by BBDM do not.}
     \label{fig:sup_PCA_Visualization}
\end{figure*}

\subsection{Additional Qualitative Results}
% We provide additional visualizations of different anatomical regions for all methods in Figures~\ref{fig:visualization_appendix_1} and \ref{fig:visualization_appendix_3}. Each visualization sample  is accompanied by corresponding error maps comparing the generated outputs to the ground truth, offering a clearer insight into the discrepancies between methods.
We provide additional visualizations of different anatomical regions for all methods in Figures~\ref{fig:visualization_appendix_1} and \ref{fig:visualization_appendix_3}. Each visualization sample is accompanied by corresponding error maps comparing the generated outputs to the ground truth, offering clearer insights into the discrepancies between methods. \figref{fig:sup_PCA_Visualization} shows more details of the PCA visualization of spatial features extracted from denoising network.

\section{Dataset Details}
All PET/CT scans are carried out at major hospitals following a consistent acquisition protocol using clinical scanners, namely the GE Discovery 710 PET/CT and GE Discovery STE PET/CT systems. The full dataset includes scans from a diverse cohort of patients, all acquired under standardized conditions to ensure consistency and comparability across the study. However, the statistical analyses presented in the following sections are based on a focused experimental subset of this dataset, specifically selected for in-depth investigation. The demographic characteristics of the patients in the experimental subset are detailed in Table \ref{tab:patient_characteristics}.

\begin{table}[t]
\centering
\caption{Patient characteristics across the experimental dataset. The values for \textbf{Age}, \textbf{Height}, and \textbf{Weight} are reported as mean ± standard deviation.}
\label{tab:patient_characteristics}
\resizebox{\linewidth}{!}{%
\begin{tabular}{l|c|c|c|c}
\toprule
\textbf{Sex} & \textbf{\# of Studies} & \textbf{Age} & \textbf{Height (m)} & \textbf{Weight (kg)} \\ 
\midrule
Male   & 333  & 59.0 ± 14.1  & 1.64 ± 0.10  & 59.6 ± 10.8 \\ 
Female & 265  & 52.8 ± 15.1  & 1.56 ± 0.09  & 53.8 ± 8.1 \\ 
\bottomrule
\end{tabular}%
}
\end{table}

For the whole-body diagnostic CT, imaging is conducted during expiration with the patient's arms raised, adhering to a standardized procedure. The tube voltage is set to 120 kVp for the GE Discovery 710 system and 140 kVp for the GE Discovery STE system, with the tube current-exposure time product automatically adjusted via automatic exposure control (AEC) to optimize image quality and radiation dose based on the anatomical region. CT images are reconstructed with a slice thickness of 3.75 mm and an in-plane voxel edge length of 0.98 mm for the GE Discovery 710 system, while for the GE Discovery STE system, the slice thickness is 5.0 mm and the voxel edge length is 1.37 mm. To convert the raw scanner data from both clinical systems into Hounsfield units (HU), a rescale slope of 1.0 and a rescale intercept of -1024.0 can be applied, ensuring accurate representation of tissue densities in the reconstructed images.

\begin{figure}[t]
    \centering
    \includegraphics[width=1.0\linewidth]{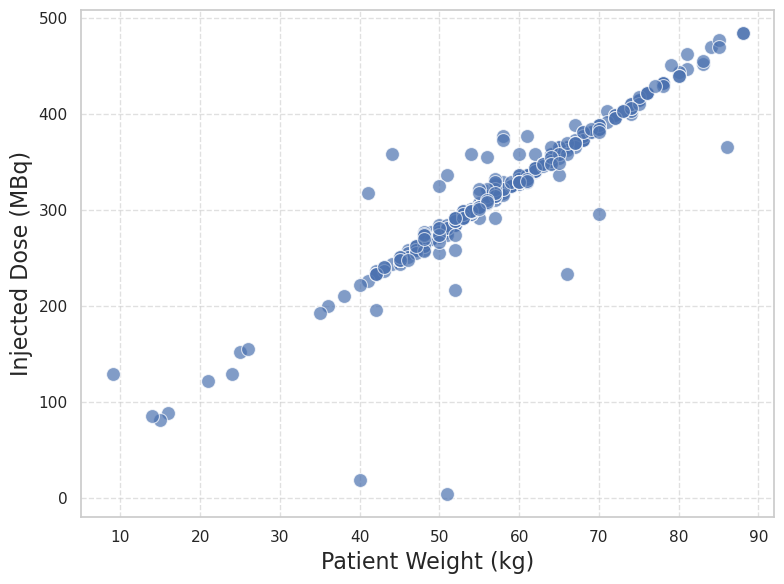}
        \caption{Correlation between Patient Weight and Injected FDG Dose.}  
   \label{fig:dose_weight}
\end{figure}

PET imaging is initiated 60 minutes after administering a weight-adjusted dose of $^{18}$F-FDG (mean: 318.4 MBq, standard deviation: 59.5 MBq, range: 3.9 – 484.7 MBq). The FDG dose is adjusted based on patient weight, as observed in the scatter plot (see Figure \ref{fig:dose_weight}), where there is a clear positive correlation between weight and injected dose. This trend suggests that the dosing strategy is influenced by patient-specific factors to ensure appropriate radiotracer distribution, likely aiming to account for variations in body mass and metabolic activity. PET scans are performed from the skull base to the mid-thigh, and the images are reconstructed using a 3D iterative algorithm. The final images have a slice thickness of 3.27 mm and a voxel edge length of 2.73 mm.
